# Supplementary material for: OLViT: Multi-Modal State Tracking via Attention-Based Embeddings for Video-Grounded Dialog
Source: arXiv:2402.13146 source file (2024-02-20)
Supplement: Supplementary file 1 [file appendix.tex]

\section{Encoder Configuration}
% We use MONet to generate $N_o=12$ object masks from each of the $T=20$ equidistantly-sampled frames from the video and DistilRoBERTa-base to generate the $d_w = 768$ dimensional word embeddings.
% Both embeddings are then mapped to a $d = 216$ dimensional space using a linear layer.

% \subsubsection{Encoder}
To find the optimal configuration of our encoder, i.e. the number transformer layers and attention heads, we conducted the following experiment while keeping all history rounds and MONet objects.
We independently optimised these two variables on the DVD dataset. 
It is worth noting that during this experiment, we also fixed number of the state tracker layers to two, i.e. $L_{ost} = L_{lst} = 2$, and used the same number of attention heads and hidden dimension $d$ as in the encoder.

\subsection{Number of Attention Heads}
\label{sec:att_heads}
 First, we fixed the number of transformer layers to four and varied the number of attention heads from two to six, thus varying the hidden dimension $d$ from $72$ to $216$ in $36$ steps. As can be seen from the first section of \autoref{tab:num_heads}, our \olvit\, model achieves the best validation accuracy of $54.01\%$ when using six attention heads corresponding to a hidden dimension $d=216$.

\subsection{Number of Transformer Layers}
\label{sec:num_layers}
 Then, we doubled the number of transformer layers starting from 4 until 16  while keeping the optimal values of the attention heads and hidden dimension fixed. As illustrated in the second section of \autoref{tab:num_heads}, the performance of \olvit\, on DVD started to decrease with more transformer layers, i.e. from $54.01\%$ validation accuracy with four layers to only $52.89\%$ with $16$ layers. This finding was expected as increasing the complexity of the model renders it more prone to over-fitting.

%and fed into the encoder or encoder/decoder block depending on the setting (discriminative vs generative).
% Both encoder and decoder have $L=4$ layers with six attention heads; all other transformer blocks have two layers and six attention heads (see \autoref{sec:encoder_config} and \ref{sec:app_num_att_layers}).
%In the discriminative setting, we minimize the cross-entropy loss over the DVD classes using a linear layer on the final [CLS] embeddings.
%In the generative setting, the model learns to predict the next token in the answer based on the context and the previous answer tokens.
% In the generative setting, we use right masking in the attention operation for the model not to have access to future answer tokens.
% During training we optimize the model weights using AdamW \cite{adamw} with an initial learning rate of $1e^{-4}$ with warm-up and cosine-decay until convergence.  
% While testing in the generative setting, we generate answers until the <EOS> token is predicted or if a maximum length of $40$ tokens is reached.

\section{State Tracker Configuration}
% We experimented with three variants of our combiner (see \autoref{fig:combiner}): Besides the transformer based approaches (see Figures \ref{fig:ost} and \ref{fig:lst}), we tried to process the DST's input using a $2-$layered LSTM with a hidden dimension of $216$.
% We considered these two variables independently and optimised them separately.
% To this end, we trained OLViT on DVD while keeping all history rounds and object embeddings obtained from MONet in LST and OST, respectively.
% We experimented with three variants of our combiner as illustrated in \autoref{fig:combiner}.
% Besides the transformer-based state tracker approaches
% % (see Figures \ref{fig:ost} and \ref{fig:lst})
% , we tried updating the state vectors using a $2$-layered LSTM \cite{lstm} with a hidden dimension of $216$.
% We considered these two variables (combiner vs. state tracker types) independently and optimised them separately.
% To this end, we trained \olvit\, on DVD while keeping all history turns and object embeddings obtained from MONet in LST and OST, respectively.

To optimise our transformer-based state trackers, we experimented with different configurations mainly varying the number of transformer layers $L_{ost}$ and $L_{lst}$ while inheriting the previous optimal values of the encoder hyper-parameters, i.e. $L=4$ and $d=216$. 
For both state trackers, we used the same number of transformer layers, i.e. $L_{ost} = L_{lst}$.
As can be seen from \autoref{tab:num_layers_tracker}, our model achieved the best DVD validation accuracy of $54.01\%$ when using two layers and its performance started to decrease with more layers reaching $53.83\%$ with $L_{ost}=L_{lst}=4$.
Similarly to the previous experiment, this finding was expected as increasing the number of state tracker layers makes the model more prone to over-fitting.
% \begin{table}[!t]
% \centering
% \scalebox{0.8}[0.8]{

% \begin{tabular}{|cccc|}
% \hline
% \textbf{\# of layers}&
% % \multirow{2}*{\textbf{\# of layers}}&
% % \multicolumn{2}{|c}{\textbf{State Trackers}} \\
%  \textbf{\# of attention } & \textbf{Hidden dim.}  & \textbf{Accuracy} \\
%  $\mathbf{L}$ & \textbf{heads} & $\mathbf{d}$   & \textbf{[\%]} \\
% \hline
% \hline
% % \multirow{4}*{\rotatebox{90}{\textbf{DVD}}} &
% {$4$}&$2$ & $72$  &  $52.63$ \\
% {$4$}&$4$ & $144$ &  $53.74$ \\
% {$\mathbf{4}$}&$\mathbf{6}$ & $\mathbf{216}$ &  $\mathbf{54.01}$ \\
% \hline
% \hline
% {$\mathbf{4}$}&$\mathbf{6}$ & $\mathbf{216}$ &  $\mathbf{54.01}$ \\
% {$8$}&$6$ & $216$ &  $53.15$ \\
% {$16$}&$6$ & $216$ &  $52.89$ \\
% \hline

% \end{tabular}
% }
% \caption{Performance comparison of our model with different number of encoder transformer layers $L$, attention heads, and embedding dimensions $d$. Performance is measured on the DVD \textit{val} split.
% The best configuration is highlighted in bold.}
% \label{tab:num_heads}
% \end{table}

\begin{table}[!t]
\centering
\scalebox{0.76}[0.76]{

\begin{tabular}{|ccccc|}
\hline
&\textbf{\# of layers}&
% \multirow{2}*{\textbf{\# of layers}}&
% \multicolumn{2}{|c}{\textbf{State Trackers}} \\
 \textbf{\# of attention } & \textbf{Hidden dim.}  & \textbf{Accuracy} \\
 & $\mathbf{L}$ & \textbf{heads} & $\mathbf{d}$   & \textbf{[\%]} \\
\hline
\hline
% \multirow{4}*{\rotatebox{90}{\textbf{DVD}}} &
\multirow{3}*{\rotatebox{90}{\ref{sec:att_heads}}}  
&\multicolumn{1}{|c}{$4$}&$2$ & $72$  &  $52.63$ \\
&\multicolumn{1}{|c}{$4$}&$4$ & $144$ &  $53.74$ \\
&\multicolumn{1}{|c}{$\mathbf{4}$}&$\mathbf{6}$ & $\mathbf{216}$ &  $\mathbf{54.01}$ \\
\hline
\hline
\multirow{3}*{\rotatebox{90}{\ref{sec:num_layers}}}
&\multicolumn{1}{|c}{$\mathbf{4}$}&$\mathbf{6}$ & $\mathbf{216}$ &  $\mathbf{54.01}$ \\
&\multicolumn{1}{|c}{$8$}&$6$ & $216$ &  $53.15$ \\
&\multicolumn{1}{|c}{$16$}&$6$ & $216$ &  $52.89$ \\
\hline
\end{tabular}
}
\caption{Performance comparison of our model with different number of encoder transformer layers $L$, attention heads, and embedding dimensions $d$. The best configuration is highlighted in bold. Performance is measured on the DVD \textit{val} split.}
\label{tab:num_heads}
\end{table}

% \subsubsection{Combiner}
% As can be seen from \autoref{fig:plots} (left), variant A of the combiner -- despite having the simplest architecture -- outperforms all other variants with a validation accuracy of $54.01\%$ on DVD.
% We hypothesise that this is because concatenating the states vectors to all respective embeddings (variant B) prevents the model from applying attention over the raw state vectors that contain rich information about the previous relevant objects and dialog turns. On the other hand, using additional transformer layers increases complexity and the risk of over-fitting (variant C).
% %as it reached a validation accuracy of merely $53.08\%$.
% The LSTM-based state tracker reached a validation accuracy of $53.20\%$ compared to $54.01\%$ achieved by the transformer-based state trackers.
% %one as can be seen in the blue plot of \autoref{fig:plots} (left).
% Therefore, in all evaluations that follow, we use variant A of the combiner and the transformer-based state trackers.
\begin{table}[!t]
\centering
\scalebox{0.79}[0.79]{

    \begin{tabular}{|cccc|}
        \hline
        \multirow{2}*{$\mathbf{L_{ost}} = \mathbf{L_{lst}}$}&
         \textbf{\# of attention } & \textbf{Hidden dim.} & \textbf{Accuracy} \\
         & \textbf{heads} & $\mathbf{d}$ & \textbf{[\%]} \\
        \hline
        \hline
        $1$ & $6$ & $216$ & $53.20$ \\
        $\mathbf{2}$ & $\mathbf{6}$ & $\mathbf{216}$ & $\mathbf{54.01}$ \\
        $3$ & $6$ & $216$ & $53.91$ \\
        $4$ & $6$ & $216$ & $53.83$ \\
        
        \hline
        
    \end{tabular}
}
\caption{Performance comparison of our model with different number of state tracker transformer layers $L_{ost}$ and $L_{lst}$.
 Performance is measured on the DVD \textit{val} split.
The best configuration is highlighted in bold.
}
\label{tab:num_layers_tracker}
\end{table}

\section{Effect of Pre-trained Language Models}
\label{sec:app_full_roberta}
To assess the effect of pre-trained language models on \olvit, we ran the following experiment. First, we completely removed the DistillRoBERTa model and trained the encoder layers from scratch.
Then, we increased the number of encoder transformer layers from 4 to 16 to compensate for the removal of the pre-trained language model.
As can be seen from \autoref{tab:lm}, our model's DVD validation accuracy dropped from $55.41\%$ to $54.46\%$ when DistillRoBERTa was removed.
However, its performance improved when we increased the number of encoder layers to 16 and reached a validation accuracy of $54.54\%$.
Finally, using a full RoBERTa model only improved the model's accuracy by $0.02\%$.
As a result, we decided to use a DistillRoBERTa model in order to train efficiently.

\section{Training Details}
We implemented our model in PyTorch \cite{pytorch} and conducted our experiments on two NVIDIA Tesla V100-SXM2-32GB GPUs and used MONet to generate
$N_o=12$ object masks from $T=20$ equidistantly-sampled frames and DistilRoBERTa-base to generate the $d_w = 768$ dimensional word embeddings.
During training, we optimised the model weights using AdamW \cite{adamw} with a batch size of $50$. We set the initial learning rate to $1e^{-4}$ and used a learning rate schedule with warm-up for $4$k iterations and cosine-decay until convergence for a total of $200$K iterations.

\begin{table}[!t]
\centering
\scalebox{0.83}[0.83]{

\begin{tabular}{|l|ccc|}
\hline

\multirow{2}*{\textbf{LM}}& \textbf{\# of LM} & \textbf{\# of Layers} & \textbf{Accuracy} \\
                           & \textbf{param.} & $\mathbf{L}$ & \textbf{[\%]} \\
\hline
\hline
None & - & $4$ & $54.46$ \\
None & - & $16$ & $54.54$ \\
\hline
\hline
DistillRoBERTa & $81.5$M & $4$ & $55.39$ \\
RoBERTa & $354$M & $\mathbf{4}$ & $\mathbf{55.41}$ \\

\hline
\end{tabular}
}
\caption{The effect of pre-trained language models on the performance of our model.
The best performance on the DVD \textit{val} split is in bold.
}
\label{tab:lm}
\end{table}
